# Supplementary material for: Cancer Metastasis: Collective Invasion in Heterogeneous Multicellular Systems
Source: arXiv:1501.00065 source file (2014-12-31)
Supplement: Supplementary file 1 [file Supplementary_Materials.pdf]

# Supplementary Materials

## Cancer Metastasis: Collective Invasion in Heterogeneous Multicellular Systems

Adrien Hallou, Joel Jennings and Alexandre Kabla

*Department of Engineering, University of Cambridge, Cambridge, CB2 1PZ, UK.*

December 31, 2014

| Cells Motile Force (μ) | | | → μ=μc | → μ=μs | → |
|---|---|---|---|---|---|
| **Type of Tissue** | **Type of Cells** | **State of the Tissue / Measured Quantity** | **Cohesive** | **Collective** | **Individual** |
| Single Cell | Motile Cell | Mean Square Displacement | ~0 | ~0 | Large |
| Homogeneous Epithelial Tissue | Motile Cells | Spatial Correlations | Low | High | Low |
| | | Temporal Correlations | Subdiffusive | Hyperdiffusive | Diffusive |
| Homogeneous Tumour | Cancer Cells | Invasion Rate | ~0 ① | Slow ② | Fast ③ |
| Heterogeneous Tumour | Cancer Cells Fibroblast Cells | Invasion Rate | ~0 ④ | Fast ⑤ | Fast ⑥ |

Table 1: Summary table linking single cell and population level behaviours (using results from [1]) with the invasion dynamics obtained for homogeneous and heterogeneous tumours.

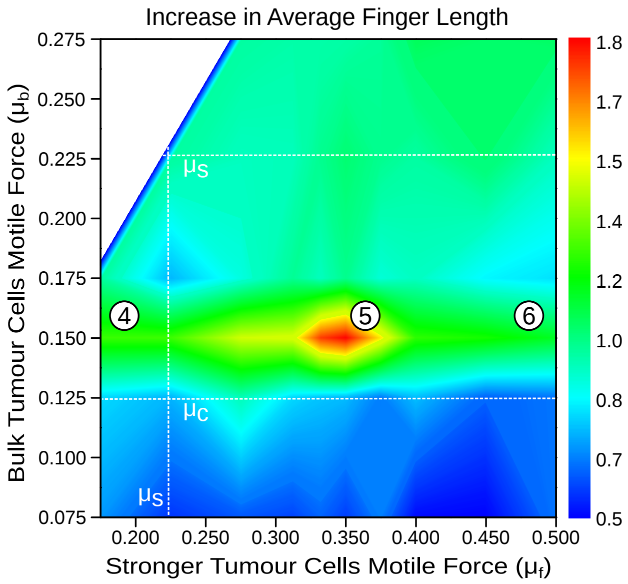


Figure 1: Heat map of the increase in average finger length with respect to $\mu_b$ and $\mu_f$. Measurements are taken on five time points between 3500 and 4500 MCS and averaged for each on 12 different runs. Data set is the same as for Fig.2.b of the main article.

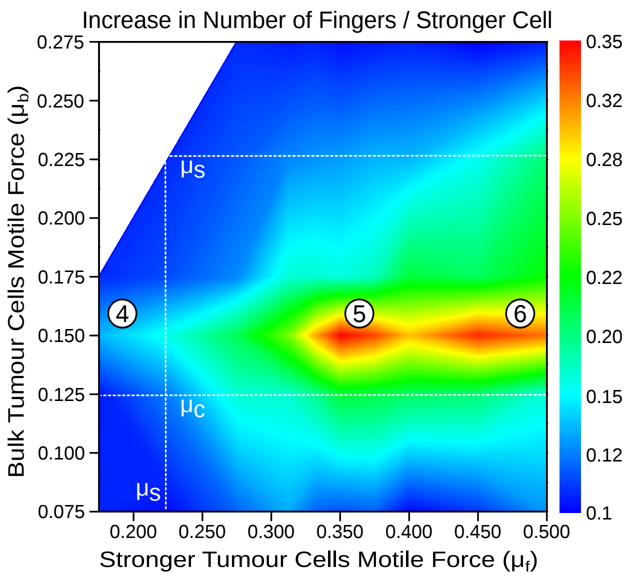


Figure 2: Heat map of the increase in number of fingers per stronger cell with respect to $\mu_b$ and $\mu_f$. Measurements are taken on five time points between 3500 and 4500 MCS and averaged for each on 12 different seeds. Data set is the same as for Fig.2.b. of the main article.

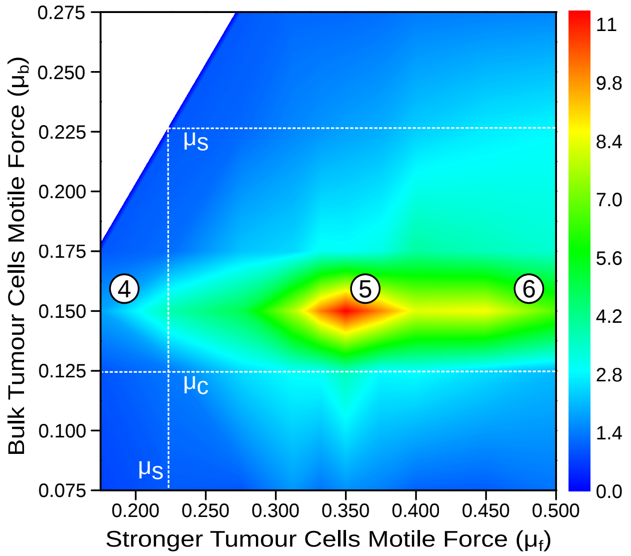


Figure 3: Heat map of the product of the increase in average finger length per the increase in number of fingers per stronger cell with respect to $\mu_b$ and $\mu_f$. Measurements are taken on five time points between 3500 and 4500 MCS and averaged for each on 12 different seeds. Data set is the same as for Fig.2.b. of the main article.

# Movies of *in silico* Experiments

The table below provides a list of all the movies cited in the main article with corresponding captions and external links to the files. The frame rate corresponds to one frame every 10 Monte-Carlo step.

| **Name of the Movie** | $N_f$ | $\mu_b$ | $\mu_f$ | **Description** |
|---|---|---|---|---|
| movie 1 | 0 | 0.275 | — | Tumour Invasion at high motile force, with predominance of single cell like invasion. |
| movie 2 | 0 | 0.075 | — | No invasion at low motile force - epithelium like dynamics. |
| movie 3 | 0 | 0.150 | — | Collective invasion of bulk tumour cells at intermediate motile force ($\mu_c < \mu_b < \mu_s$). |
| movie 4 | 24 | 0.150 | 0.500 | High heterogeneity in motile strength. Stronger cells invade rapidly but fail to trigger collective invasion. Bulk tumour cells invasion remains weak as a result. |
| movie 5 | 24 | 0.125 | 0.175 | Low heterogeneity and low motile force. Slow collective invasion of bulk tumour cells and no stronger cell led fingers since $\mu_f < \mu_s$. |
| movie 6 | 24 | 0.150 | 0.350 | Optimum of stronger cell led invasion. Both tumour cell types co-invade through long and numerous finger like protrusions with stronger cells at their leading edge. |


[1] A.J. Kabla, Journal of The Royal Society Interface **9**, 3268(2012).
